# Supplementary material for: Stable Machine Learning Potentials for Liquid Metals via Dataset Engineering
Source: arXiv:2601.05003 ancillary file (2026-01-08)
Supplement: Supplementary file 1 [file supplementary_information.pdf]

# Supplementary Information

**Stable Machine Learning Potentials for Liquid Metals via Dataset Engineering**

Alex Tai[1], Jason Ogbebor[1], Rodrigo Freitas[1*]
[1] *Department of Materials Science and Engineering, Massachusetts Institute of Technology, MA, USA*

## Table of contents

**Supplementary Section 1: Derivation of the relationship between $\alpha$ and the Lindemann criterion** . **2**
**Supplementary Section 2: Coverage of configuration space in AIMD** . . . . . . . . . . . . . . . . . . . . **3**
**Supplementary Section 3: Dependence of liquid properties on $\alpha$** . . . . . . . . . . . . . . . . . . . . . . . . **4**
**Supplementary Section 4: Summary of SL training datasets** . . . . . . . . . . . . . . . . . . . . . . . . . . **5**
**Supplementary Section 5: Energy mean absolute errors** . . . . . . . . . . . . . . . . . . . . . . . . . . . . **6**
**Supplementary Section 6: Density plots with legends** . . . . . . . . . . . . . . . . . . . . . . . . . . . . . **7**
**Supplementary Section 7: Summary of calculated liquid-phase properties** . . . . . . . . . . . . . . . . . **9**
**Supplementary Section 8: Error in the melting temperature** . . . . . . . . . . . . . . . . . . . . . . . . . **10**
**Supplementary Section 9: Icosahedral ordering in the liquid phase** . . . . . . . . . . . . . . . . . . . . **11**

*Corresponding author (`rodrigof@mit.edu`).

**Supplementary Section 1: Derivation of the relationship between $\alpha$ and the Lindemann criterion**

In the SL approach, thermal noise is modeled by randomly displacing atoms from their ideal lattice positions uniformly within a spherical volume. The radius of this sphere, $R$, is controlled by the parameter $\alpha$. The parameter is defined such that $\alpha = 1$ corresponds to a radius extending halfway to the nearest-neighbor distance, $d$ (i.e., the touching limit for non-overlapping hard spheres). Thus, the maximum displacement radius of an atom for a given $\alpha$ is:

$$R = \alpha \left( \frac{d}{2} \right). \tag{1}$$

To relate this geometric parameter to the Lindemann criterion[1], we calculate the mean squared displacement, $\langle \mu^2 \rangle$, of an atom uniformly distributed within this sphere. For a sphere of radius $R$ with uniform probability density, the expectation value is:

$$\langle \mu^2 \rangle = \frac{\int_0^R r^2 (4\pi r^2)\, \mathrm{d}r}{\int_0^R (4\pi r^2)\, \mathrm{d}r} = \frac{4\pi \left[ \frac{r^5}{5} \right] \Big|_0^R}{\frac{4}{3}\pi R^3} = \frac{3}{R^3} \left( \frac{R^5}{5} \right) = \frac{3}{5} R^2. \tag{2}$$

The Lindemann melting criterion relates melting to the point where the root-mean-square vibrational amplitude reaches a critical fraction, $\eta$ (the Lindemann coefficient), of the nearest-neighbor distance:

$$\sqrt{\langle \mu^2 \rangle} = \eta d. \tag{3}$$

Substituting eq. (2) and eq. (1) into the Lindemann condition in eq. (3), we obtain:

$$\sqrt{\frac{3}{5} \left( \frac{\alpha d}{2} \right)^2} = \eta d. \tag{4}$$

Squaring both sides and simplifying yields:

$$\frac{3}{5} \left( \frac{\alpha^2 d^2}{4} \right) = \eta^2 d^2 \tag{5}$$

$$\frac{3}{20} \alpha^2 = \eta^2. \tag{6}$$

Solving for $\alpha$, we recover the direct relationship between the disorder parameter and the Lindemann coefficient:

$$\alpha = \sqrt{\frac{20}{3}} \eta, \tag{7}$$

which is eq. 2 in the main text.

**Supplementary Section 2: Coverage of configuration space in AIMD**

Here we present the coverage of configuration space sampled by AIMD trajectories using polar representations analogous to fig. 2b of the main text, which shows same analysis for the SL training set for different values of $\alpha_{\max}$. Supplementary fig. 1 shows distributions obtained from AIMD snapshots at three representative temperatures: 500 K, 1500 K, and 2500 K. While increasing temperature broadens the distribution, the overall extent of configuration space sampled by AIMD changes only modestly. In particular, raising the AIMD temperature from 1500 K to 2500 K does not visibly extend coverage toward shorter interatomic distances.

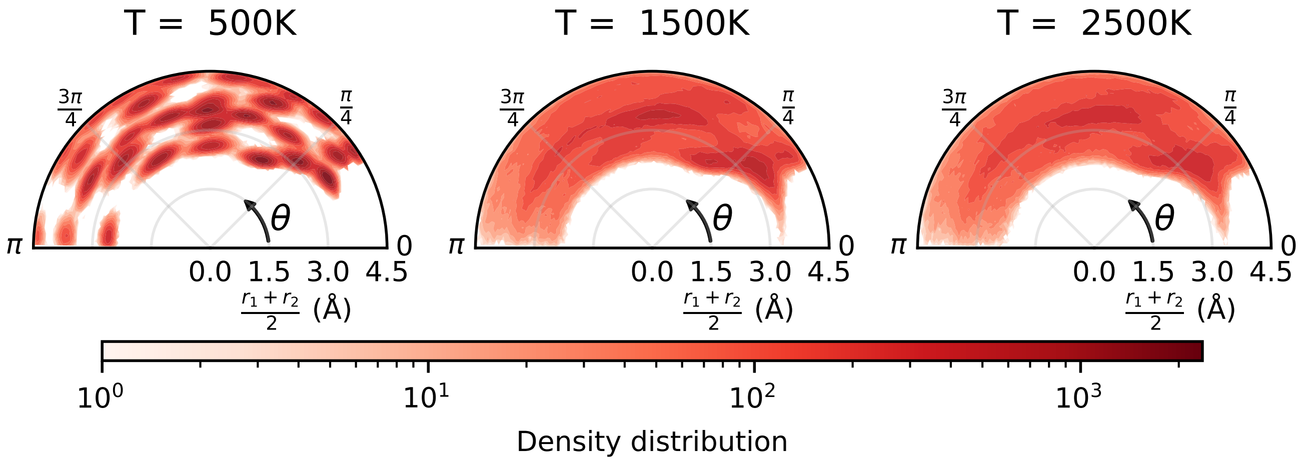


**Supplementary Figure 1:** Coverage of configuration space by snapshots from AIMD trajectories at 500 K, 1500 K, and 2500 K.

The primary distinction between AIMD (supplementary fig. 1) and SL (fig. 2b of the main text) sampling lies in the treatment of these short-range configurations. As discussed in fig. 1e in the main text, SL datasets explicitly include short interatomic distances and low-angle triplets that are rare or absent in AIMD trajectories, even at elevated temperatures. These regions correspond to the tails of the configuration-space distribution, which are sparsely populated in AIMD due to the strong energetic penalties associated with close atomic encounters. In large-scale production MD simulations, where both system size and trajectory length are substantially increased, such configurations are inevitably encountered. When these undersampled regions are reached, MLPs trained solely on AIMD data produce unphysical force predictions, leading to the instabilities observed in the figs. 1a and 1b of the main text. The SL approach addresses this limitation by deliberately populating these sparsely sampled regions of configuration space during training, thereby stabilizing MD trajectories at high temperatures and large system sizes.

**Supplementary Section 3: Dependence of liquid properties on $\alpha$**

The variations of liquid density and diffusivity with $\alpha_{\mathrm{max}}$ at 1700 K and 2000 K are shown in supplementary figs. 2a and 2b, respectively. The results show no clear trend with $\alpha_{\mathrm{max}}$, demonstrating that even with high values of $\alpha_{\mathrm{max}}$, potentials do not become overly repulsive. In contrast, MLPs with $\alpha_{\mathrm{max}} < 0.55$ tend to produce higher densities and lower diffusivities, indicating that datasets lacking sufficient coverage of shorter-range interactions yield MLPs that are insufficiently repulsive at short distances. This effect becomes more pronounced at higher temperatures, where shorter interatomic distances are more common.

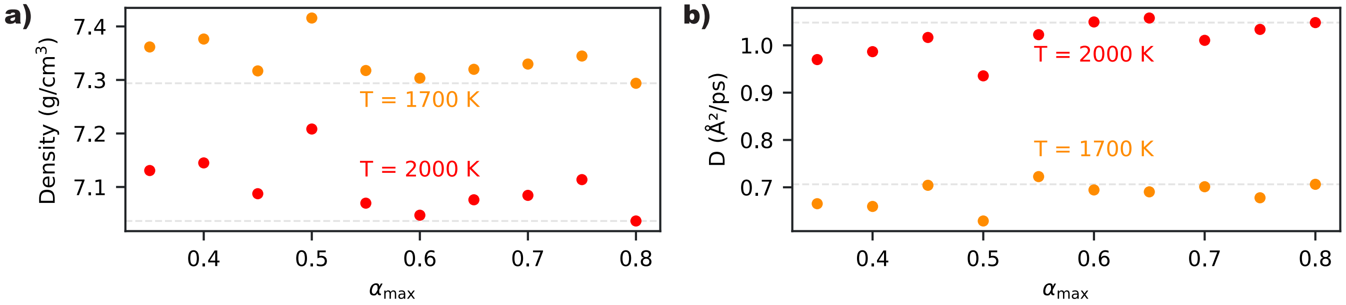


**Supplementary Figure 2:** Density and diffusivity calculated by potentials trained on datasets with varying levels of thermal noise.

## Supplementary Section 4: Summary of SL training datasets

Supplementary Table 1 summarizes the training datasets used for the calculation of liquid properties reported in fig. 4 of the main text. For each element, datasets were constructed following the synthetic-liquid (SL) procedure described in the Methods, with identical parameters used for the PBE and r$^2$SCAN exchange–correlation functionals to enable direct comparison.

The table reports the reference crystal structures used to generate perturbed configurations, the number of atoms per structure, the number of distinct structures included in each dataset, the maximum displacement amplitude $\alpha_{\mathrm{max}}$, and the total number of atoms represented. For elements whose ground-state structure is not fcc (Mg, Ti, Mo, and W), datasets include both the ground-state structure and fcc-based configurations. The inclusion of fcc environments reflects the close geometric relationship between fcc coordination and the quasi-icosahedral local order characteristic of metallic liquids, ensuring consistent sampling of liquidlike local environments across elements. All datasets employ a consistent value of $\alpha_{\mathrm{max}} = 0.6$, corresponding to the regime identified in the main text as sufficient to capture short-range interactions relevant to liquid stability and transport.

| **Element** | **Base structure** | **Atoms per structure** | **Structures** | $\alpha_{\mathbf{max}}$ | **Total atoms** |
|---|---|---|---|---|---|
| Ni | FCC | 48 | 50 | 0.6 | 2400 |
| Al | FCC | 48 | 50 | 0.6 | 2400 |
| Co | FCC | 48 | 50 | 0.6 | 2400 |
| Mg | HCP | 54 | 25 | 0.6 | 2550 |
| | FCC | 48 | 25 | 0.6 | |
| Ti | HCP | 54 | 25 | 0.6 | 2550 |
| | FCC | 48 | 25 | 0.6 | |
| Mo | BCC | 54 | 25 | 0.6 | 2550 |
| | FCC | 48 | 25 | 0.6 | |
| W | BCC | 54 | 25 | 0.6 | 2550 |
| | FCC | 48 | 25 | 0.6 | |

**Supplementary Table 1:** Dataset parameters and structures.

## Supplementary Section 5: Energy mean absolute errors

Supplementary fig. 3 shows the mean absolute error (MAE) of energy predictions for structures extracted from *ab initio* molecular dynamics (AIMD) trajectories. Compared to force errors (fig. 2c in the main text), the energy MAE exhibits noticeably higher statistical noise. This difference arises from the substantially smaller number of independent energy data points: each structure contributes a single total energy, whereas force errors are evaluated over three Cartesian components per atom, yielding 324 force components for a 108-atom structure.

Statistical uncertainty in the energy MAE was estimated using the same bootstrap resampling procedure employed for force-error analysis in the main text (fig. 2c). For each bootstrap iteration, data points were randomly drawn with replacement from the original dataset until a sample of equal size was obtained, and the MAE was computed for the resampled dataset. Vertical error bars represent the standard deviation of the MAE obtained from 100 independent bootstrap realizations.

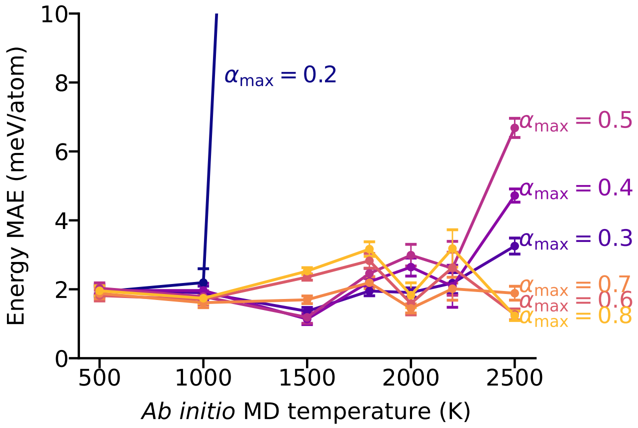


**Supplementary Figure 3:** Mean absolute error on energy predictions of structures taken from *ab initio* molecular dynamics.

## Supplementary Section 6: Density plots with legends

Figure 4a of the main text presents experimental data on liquid density in black to avoid visual clutter, despite the data originating from many independent sources. Here, we reproduce the corresponding per-element density plots using color to distinguish individual experimental datasets, with complete reference information provided in the figure captions.

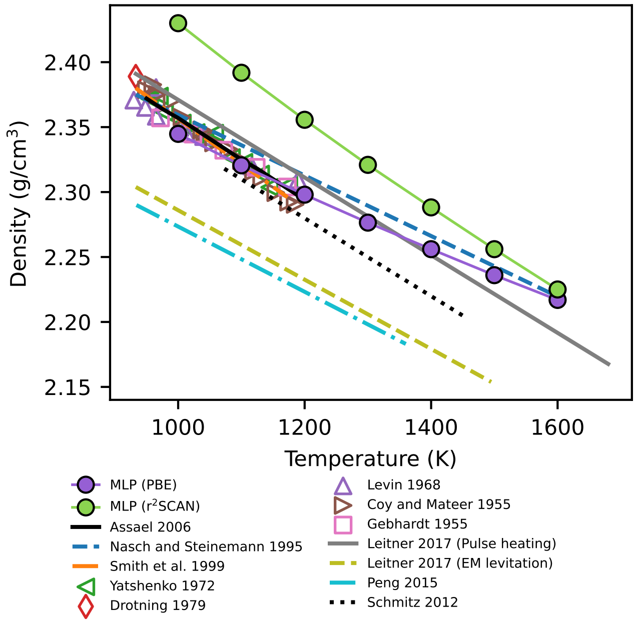


**Supplementary Figure 4:** Aluminum[2–12].

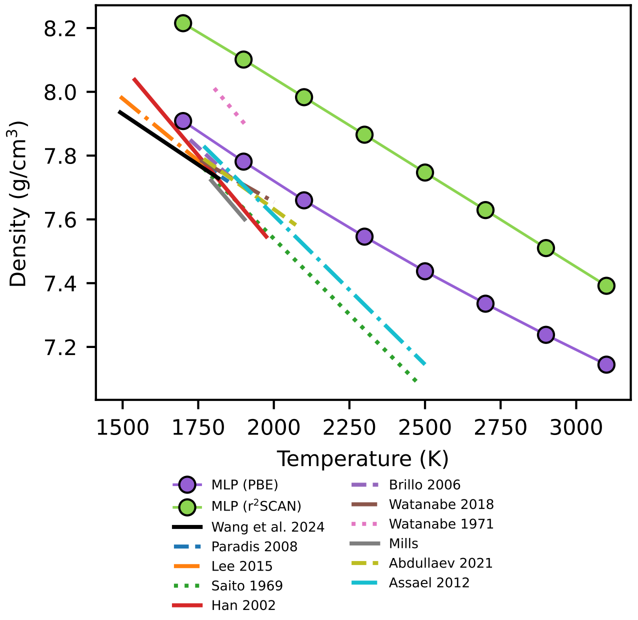


**Supplementary Figure 5:** Cobalt[13–23].

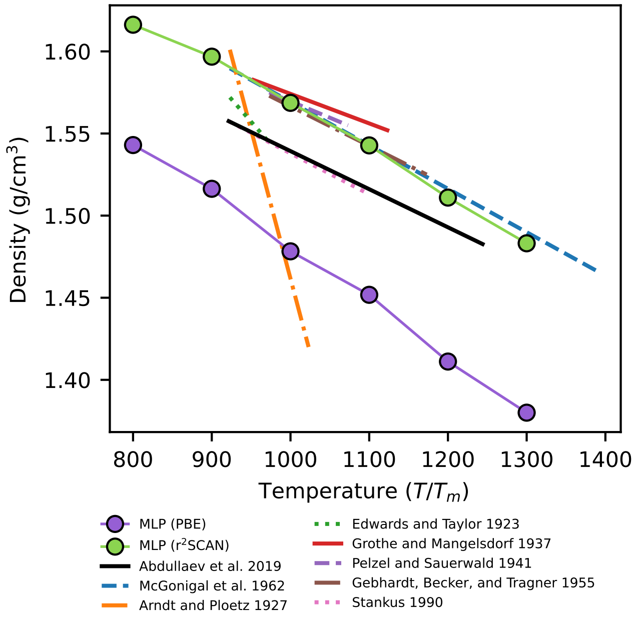


**Supplementary Figure 6:** Magnesium[24–31].

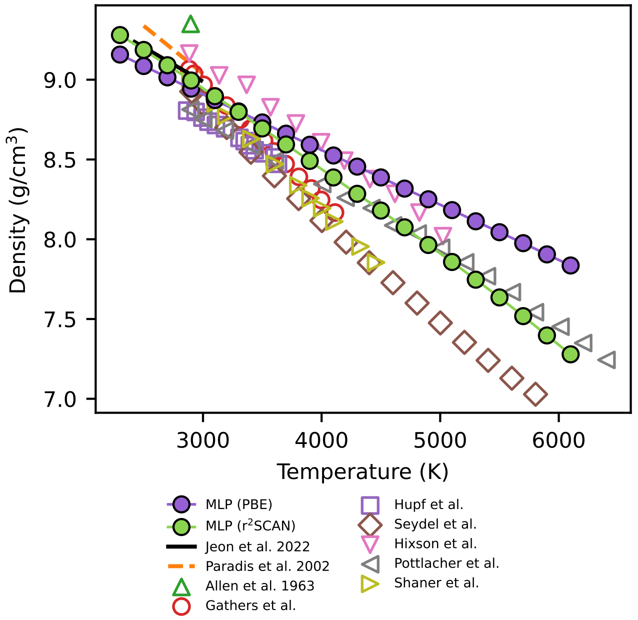


**Supplementary Figure 7:** Molybdenum[32–37].

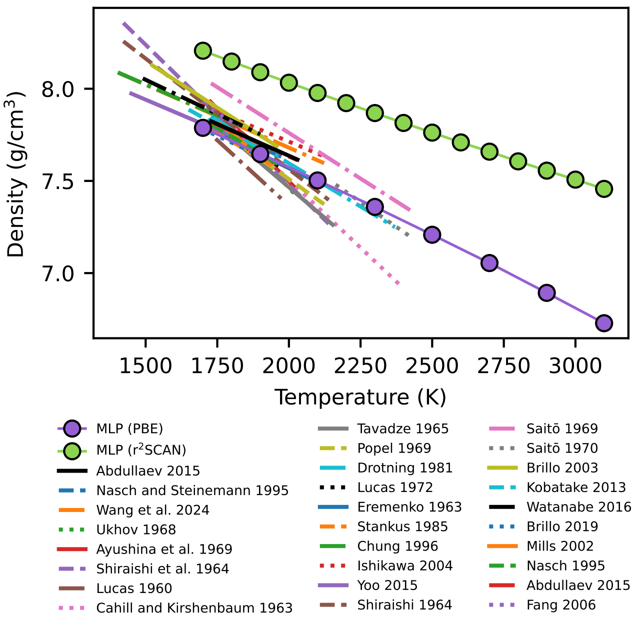


**Supplementary Figure 8:** Nickel[5,13,16,21,38–58].

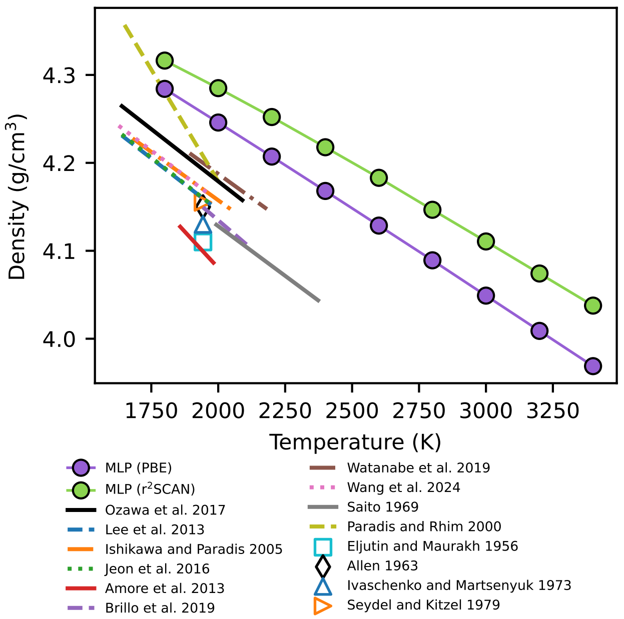


**Supplementary Figure 9:** Titanium[13,16,36,57,59–66].

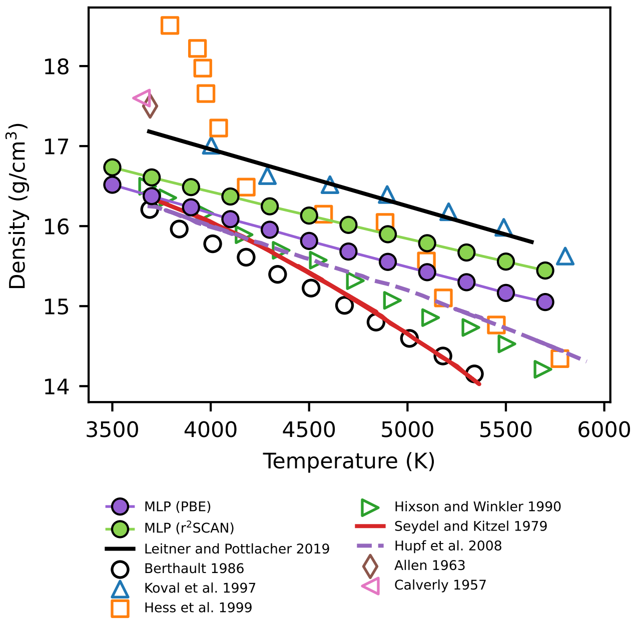


**Supplementary Figure 10:** Tungsten[34,36,67–73].

**Supplementary Section 7: Summary of calculated liquid-phase properties**

Supplementary Table 2 summarizes the transport and thermodynamic properties of the liquid metals calculated using PBE and r$^2$SCAN trained MLPs. The parameters listed are defined as follows:

- $T_\mathrm{m}$: the calculated melting temperature.
- $\rho_{T_\mathrm{m}}$: the density of the liquid phase at the melting temperature.
- $\beta$: the temperature coefficient of density. This parameter defines the linear dependence of liquid density on temperature according to the relation $\rho(T) = \rho_{T_\mathrm{m}} + \beta(T - T_\mathrm{m})$.
- $D_0$: the pre-exponential factor for self-diffusion. This is derived from fitting the calculated self-diffusion coefficients to the Arrhenius equation, $D(T) = D_0 \exp(-\Delta E/k_B T)$.
- $\Delta E$: the activation energy for self-diffusion, representing the energy barrier for atomic motion in the liquid state.

| **System** | **Functional** | $T_\mathrm{m}$ (K) | $\rho_{T_\mathrm{m}}$ (g/cm$^3$) | $\beta$ (10$^{-4}$ g/cm$^3$.K) | $D_0$ (10$^{-4}$ cm$^2$/s) | $\Delta E$ (eV) |
|---|---|---|---|---|---|---|
| Cu | PBE | 1256 | 7.685 | 8.563 | 8.01 | 0.356 |
| | r$^2$SCAN | 1365 | 8.042 | 7.946 | 7.84 | 0.381 |
| Ni | PBE | 1634 | 7.852 | 7.548 | 12.88 | 0.514 |
| | r$^2$SCAN | 1738 | 8.176 | 5.340 | 10.65 | 0.516 |
| Al | PBE | 915.6 | 2.360 | 2.124 | 7.84 | 0.211 |
| | r$^2$SCAN | 1075.6 | 2.401 | 3.408 | 13.26 | 0.289 |
| Ti | PBE | 1824.9 | 4.281 | 1.973 | 13.47 | 0.546 |
| | r$^2$SCAN | 2002.8 | 4.285 | 1.751 | 14.00 | 0.597 |
| Mg | PBE | 857.9 | 1.527 | 3.305 | 19.97 | 0.283 |
| | r$^2$SCAN | 1103.7 | 1.539 | 2.711 | 22.98 | 0.345 |
| Co | PBE | 1756 | 7.858 | 5.444 | 11.70 | 0.540 |
| | r$^2$SCAN | 1933 | 8.082 | 5.894 | 12.04 | 0.596 |
| Mo | PBE | 2908 | 8.936 | 3.443 | 16.88 | 0.861 |
| | r$^2$SCAN | 3135 | 8.892 | 5.234 | 19.60 | 0.898 |
| W | PBE | 3730.5 | 16.315 | 6.462 | 13.16 | 1.033 |
| | r$^2$SCAN | 3846.3 | 16.506 | 5.726 | 14.61 | 1.113 |

**Supplementary Table 2:** Liquid metal properties calculated using PBE- and r$^2$SCAN-based potentials.

**Supplementary Section 8: Error in the melting temperature**

To facilitate comparison across elements with widely different melting temperatures (fig. 4c of the main text), supplementary fig. 11 presents the error in the calculated melting temperature for each MLP in two complementary forms. Supplementary fig. 11a shows the absolute deviation from experiment, while supplementary fig. 11b shows the same data normalized by the experimental melting temperature (i.e., relative error). It is clear that r$^2$SCAN-trained MLPs exhibit a systematic tendency to overestimate melting temperatures across elements, whereas PBE-trained MLPs more often underestimate them. While this bias frequently results in larger absolute and relative errors for r$^2$SCAN, the magnitude of the error is element dependent, and PBE yields comparable or larger deviations for some systems. This behavior mirrors the overbinding tendency of r$^2$SCAN observed for both solid- and liquid-phase densities in the main text (fig. 5) and underscores that increased functional sophistication does not guarantee uniformly improved melting-point predictions for liquid metals.

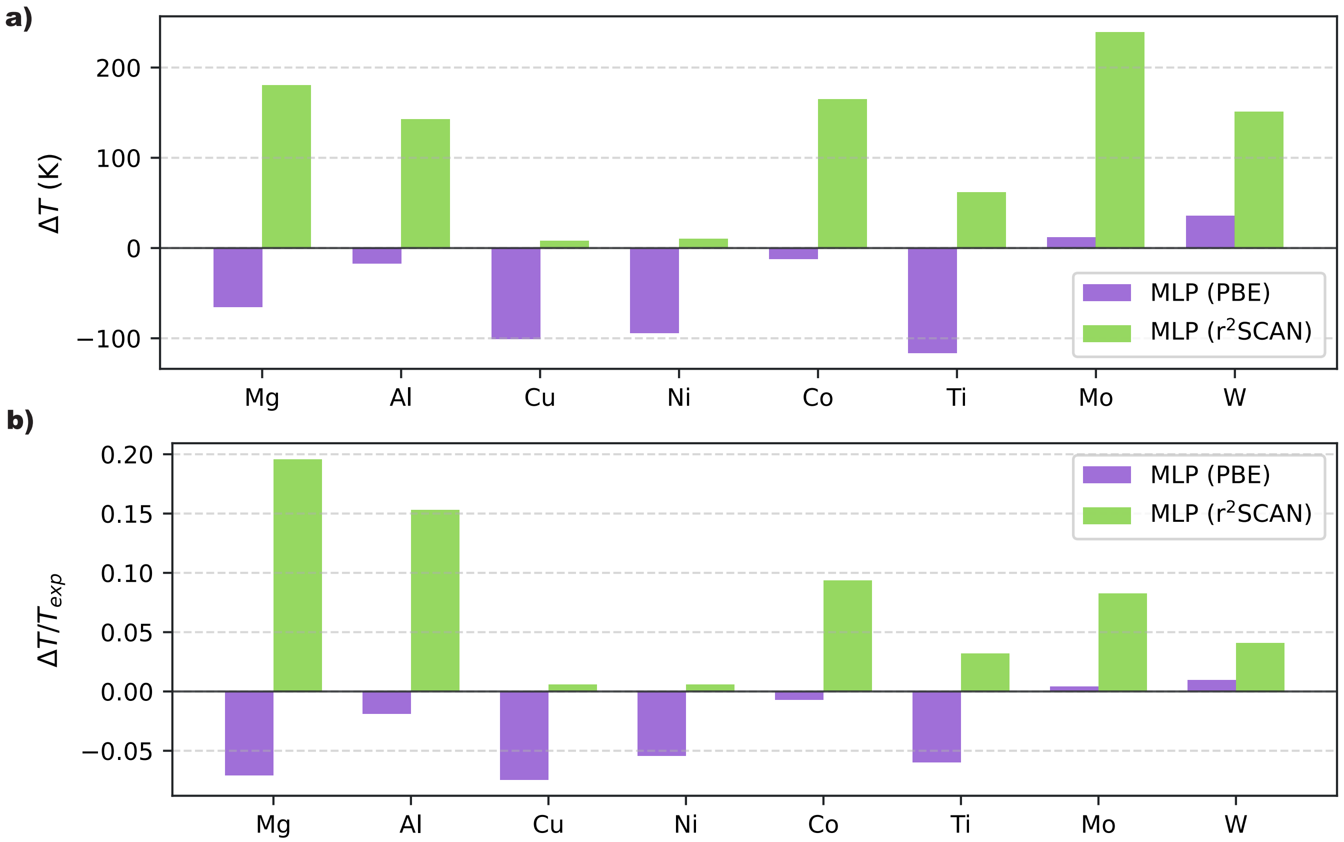


**Supplementary Figure 11:** Error on the melting point **a)** in absolute temperature and **b)** normalized by the melting point.

## Supplementary Section 9: Icosahedral ordering in the liquid phase

To illustrate the physical motivation underlying the synthetic-liquid (SL) dataset construction, we analyzed the fraction of atoms exhibiting icosahedral coordination in the liquid phase as a function of temperature for each MLP. The analysis was performed using polyhedral template matching (PTM) as implemented in OVITO[74,75]. Only atoms classified as icosahedral were retained for this analysis; all other local environments were excluded. A root-mean-square deviation threshold of 0.25 was used to identify icosahedral motifs.

Supplementary fig. 12 shows that all MLPs predict a significant population of icosahedrally coordinated atoms in the liquid phase over the temperature range considered. This observation is consistent with the well-established presence of quasi-icosahedral short-range order in metallic liquids and provides an illustration that the local structural motifs emphasized in the SL construction are also expressed in the resulting liquid configurations.

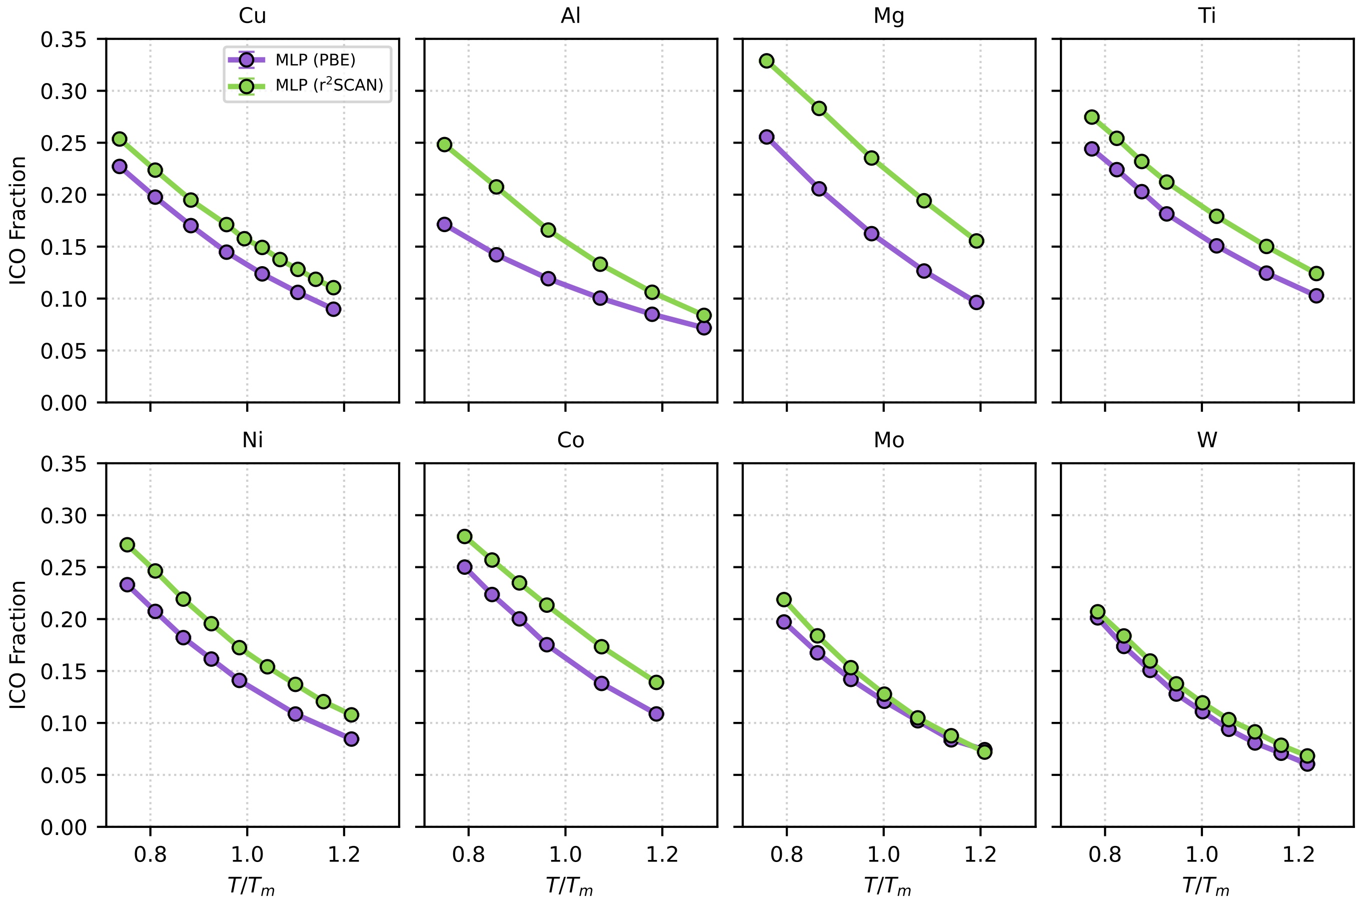


**Supplementary Figure 12:** Fraction of atoms with icosahedral order for all potentials.

## References

[1] FA Lindemann, "The calculation of molecular vibration frequencies Phys", *Physikalische Zeitschrift* (1910).

[2] Marc J. Assael, Konstantinos Kakosimos, R. Michael Banish, Jürgen Brillo, Ivan Egry, Robert Brooks, Peter N. Quested, Kenneth C. Mills, Akira Nagashima, Yuzuru Sato, and William A. Wakeham, "Reference Data for the Density and Viscosity of Liquid Aluminum and Liquid Iron", en, *Journal of Physical and Chemical Reference Data* (Mar. 2006), ISSN: 0047-2689, 1529-7845, DOI: 10.1063/1.2149380.

[3] Patrick M Smith, John W Elmer, and Gilbert F Gallegos, "Measurement of the density of liquid aluminum alloys by an x-ray attenuation technique", en, *Scripta Materialia* (Mar. 1999), ISSN: 13596462, DOI: 10.1016/S1359-6462(99)00043-3.

[4] S. P. Yatsenko, V. I. Kononenko, and A. L. Suhman, *High Temperature* (1972).

[5] P. M. Nasch and S. G. Steinemann, "Density and Thermal Expansion of Molten Manganese, Iron, Nickel, Copper, Aluminum and Tin by Means of the Gamma-Ray Attenuation Technique", en, *Physics and Chemistry of Liquids* (Jan. 1995), ISSN: 0031-9104, 1029-0451, DOI: 10.1080/00319109508030263.

[6] E. S. Levin, G. D. Ayushina, and P. V. Geld, *High Temperature* (1968).

[7] W.J. Coy and R.S. Mateer, *Transactions of the American Society for Metals* (1955).

[8] E. Gebhardt, M. Becker, and S. Dorner, *Aluminium* (1955).

[9] Matthias Leitner, Thomas Leitner, Alexander Schmon, Kirmanj Aziz, and Gernot Pottlacher, "Thermophysical Properties of Liquid Aluminum", en, *Metallurgical and Materials Transactions A* (June 2017), ISSN: 1543-1940, DOI: 10.1007/s11661-017-4053-6.

[10] H. L. Peng, Th. Voigtmann, G. Kolland, H. Kobatake, and J. Brillo, "Structural and dynamical properties of liquid Al-Au alloys", en, *Physical Review B* (Nov. 2015), ISSN: 1098-0121, 1550-235X, DOI: 10.1103/PhysRevB.92.184201.

[11] W.D. Drotning, *Thermal expansion and density measurements of molten and solid materials at high temperatures by the gamma attenuation technique*, en, tech. rep., May 1979, DOI: 10.2172/6007362.

[12] Julianna Schmitz, Bengt Hallstedt, Jürgen Brillo, Ivan Egry, and Michael Schick, "Density and thermal expansion of liquid Al–Si alloys", en, *Journal of Materials Science* (Apr. 2012), ISSN: 0022-2461, 1573-4803, DOI: 10.1007/s10853-011-6219-8.

[13] Lei Wang, Yong Chan Cho, Yun-Hee Lee, John Jonghyun Lee, and Geun Woo Lee, "Density measurement and uncertainty evaluation of elemental and alloy liquids using electrostatic levitation", en, *Journal of Molecular Liquids* (Feb. 2024), ISSN: 01677322, DOI: 10.1016/j.molliq.2024.123979.

[14] Paul-François Paradis, Takehiko Ishikawa, and Noriyuki Koike, "Thermophysical property measurements of liquid and supercooled cobalt.", *High Temperatures-High Pressures* (2008).

[15] Jonghyun Lee, Justin E. Rodriguez, Robert W. Hyers, and Douglas M. Matson, "Measurement of Density of Fe-Co Alloys Using Electrostatic Levitation", en, *Metallurgical and Materials Transactions B* (Dec. 2015), ISSN: 1543-1916, DOI: 10.1007/s11663-015-0434-7.

[16] Tunezō Saitō, Yutaka Shiraishi, and Yutaka Sakuma, "Density Measurement of Molten Metals by Levitation Technique at Temperatures between 1800° and 2200°C", en, *Transactions of the Iron and Steel Institute of Japan* (1969), ISSN: 0021-1583, 1881-1183, DOI: 10.2355/isijinternational1966.9.118.

[17] X. J Han, N Wang, and B Wei, "Thermophysical properties of undercooled liquid cobalt", en, *Philosophical Magazine Letters* (Aug. 2002), ISSN: 0950-0839, 1362-3036, DOI: 10.1080/09500830210144382.

[18] Jürgen Brillo, Ivan Egry, and Taishi Matsushita, "Density and excess volumes of liquid copper, cobalt, iron and their binary and ternary alloys", en, *International Journal of Materials Research* (Nov. 2006), ISSN: 2195-8556, 1862-5282, DOI: 10.3139/146.101415.

[19] Manabu Watanabe, Junichi Takano, Masayoshi Adachi, Masahito Uchikoshi, and Hiroyuki Fukuyama, "Thermophysical properties of liquid Co measured by electromagnetic levitation technique in a static magnetic field", en, *The Journal of Chemical Thermodynamics* (June 2018), ISSN: 00219614, DOI: 10.1016/j.jct.2018.02.004.

[20] Shunroku Watanabe, "Densities and Viscosities of Iron, Cobalt and Fe–Co Alloy in Liquid State", en, *Transactions of the Japan Institute of Metals* (1971), ISSN: 0021-4434, 2432-4701, DOI: 10.2320/matertrans1960.12.17.

[21] Kenneth C Mills, *Recommended values of thermophysical properties for selected commercial alloys*, Woodhead publishing, 2002, DOI: 10.1533/9781845690144.

[22] R. N. Abdullaev, R. A. Khairulin, Yu. M. Kozlovskii, and S. V. Stankus, "Density and Thermal Expansion of High Purity Cobalt over the Temperature Range from 140 K to 2073 K", en, *Metallurgical and Materials Transactions A* (Dec. 2021), ISSN: 1073-5623, 1543-1940, DOI: 10.1007/s11661-021-06485-1.

[23] Marc J. Assael, Ivi J. Armyra, Juergen Brillo, Sergei V. Stankus, Jiangtao Wu, and William A. Wakeham, "Reference Data for the Density and Viscosity of Liquid Cadmium, Cobalt, Gallium, Indium, Mercury, Silicon, Thallium, and Zinc", *Journal of Physical and Chemical Reference Data* (July 2012), ISSN: 0047-2689, DOI: 10.1063/1.4729873.

[24] R.N. Abdullaev, R.A. Khairulin, Yu. M. Kozlovskii, A. Sh. Agazhanov, and S.V. Stankus, "Density of magnesium and magnesium-lithium alloys in solid and liquid states", en, *Transactions of Nonferrous Metals Society of China* (Mar. 2019), ISSN: 10036326, DOI: 10.1016/S1003-6326(19)64959-9.

[25] P. J. McGonigal, A. D. Kirshenbaum, and A. V. Grosse, "THE LIQUID TEMPERATURE RANGE, DENSITY, AND CRITICAL CONSTANTS OF MAGNESIUM[1]", en, *The Journal of Physical Chemistry* (Apr. 1962), ISSN: 0022-3654, 1541-5740, DOI: 10.1021/j100810a038.

[26] Erich Gebhardt, Manfred Becker, and Erich Trägner, "Über die Eigenschaften metallischer Schmelzen: X. Die innere Reibung flüssiger Magnesium-Blei-Legierungen", *International Journal of Materials Research* (1955), DOI: 10.1515/ijmr-1955-460204.

[27] H. Grothe and C. Mangelsdorf, "The liquid temperature range, density, and critical constants of magnesium" (1937).

[28] S V Stankus and R A Khairulin, "Temperature and interphase changes in the density of magnesium in the solid and liquid states", Russian, *Tsvetnye metally* (1990).

[29] K Arndt and G Ploetz, "The density of molten magnesium", German, *Zeitschrift für Physikalische Chemie* (1927).

[30] JD Edwards and CS Taylor, "Density of magnesium from 20 to 700° C [J]", *Transactions of the AIME* (1923).

[31] E Pelzel and F Sauerwald, "Density measurements at high temperatures XII", *Zeitschrift für Metallkunde* (1941).

[32] Sangho Jeon, Shraddha Ganorkar, Yong Chan Cho, Joohyun Lee, Minju Kim, Jonghyun Lee, and Geun Woo Lee, "Precise density measurement and its uncertainty evaluation for refractory liquid metals over 3000 K using electrostatic levitation", *Metrologia* (Aug. 2022), ISSN: 0026-1394, 1681-7575, DOI: 10.1088/1681-7575/ac7688.

[33] P.-F. Paradis, T. Ishikawa, and S. Yoda, "Noncontact Measurements of Thermophysical Properties of Molybdenum at High Temperatures", *International Journal of Thermophysics* (2002), ISSN: 0195928X, DOI: 10.1023/A:1015169721771.

[34] BC Allen, "The surface tension of liquid transition metals at their melting points", *Trans. AIME* (1963).

[35] John W Shaner, G Roger Gathers, and Camille Minichino, "Thermophysical properties of liquid tantalum and molybdenum", *High Temperatures-High Pressures* (1977).

[36] U. Seydel and W. Kitzel, "Thermal volume expansion of liquid Ti, V, Mo, Pd, and W", en, *Journal of Physics F: Metal Physics* (Sept. 1979), ISSN: 0305-4608, DOI: 10.1088/0305-4608/9/9/001.

[37] D. V. Minakov, M. A. Paramonov, and P. R. Levashov, "Ab initio inspection of thermophysical experiments for molybdenum near melting", *AIP Advances* (Dec. 2018), ISSN: 2158-3226, DOI: 10.1063/1.5062152.

[38] J. Brillo and I. Egry, "Density Determination of Liquid Copper, Nickel, and Their Alloys", en, *International Journal of Thermophysics* (July 2003), ISSN: 1572-9567, DOI: 10.1023/A:1025021521945.

[39] R N Abdullaev, Yu M Kozlovskii, R A Khairulin, and S V Stankus, "Density and Thermal Expansion of High Purity Nickel over the Temperature Range from 150 K to 2030 K", en, *Int J Thermophys* (2015), DOI: 10.1007/s10765-015-1839-x.

[40] V.F. Ukhov, "Surface Properties and Density of the Palladium-Based Alloys", PhD thesis, 1968.

[41] GD Ayushina, ES Levin, and PV Gel'd, "The density and surface energy of liquid alloys of aluminium with cobalt and nickel", *Russ. J. Phys. Chem* (1969).

[42] S. Y. Shiraishi and R. G. Ward, "The Density of Nickel in the Superheated and Supercooled Liquid States", en, *Canadian Metallurgical Quarterly* (Jan. 1964), ISSN: 0008-4433, 1879-1395, DOI: 10.1179/cmq.1964.3.1.117.

[43] AD Kirshenbaum and J Cahill, "Densities of liquid nickel and cobalt and an estimate of their critical constants", *Trans. of ASM* (1963).

[44] LD Lucas, "Densite du fer, du nickel et du cobalt a l'etat liquid", *Comptes Rendus de l'Academie des Sciences* (1960).

[45] Tunezo SAITO and Yutaka SAKUMA, *Densities of Pure Iron, Cobalt and Nickel in the Molten State*, en, 1970, DOI: 10.50974/00042604.

[46] F.N. Tavadze, I.A. Bairamasvili, and D.V. Khantadze, Russian, *Surface Phenomena in Melts and in Solids Arising from the Melts*, Nalchik: Kabardino-Balkaria State University, 1965.

[47] L. Fang, F. Xiao, Y.F. Wang, Z.N. Tao, and K. MuKai, "Density and molar volume of liquid Ni–Co binary alloys", en, *Materials Science and Engineering: B* (July 2006), ISSN: 09215107, DOI: 10.1016/j.mseb.2006.02.015.

[48] SI Popel, LM Shergin, and BV Tsarevskii, *TEMPERATURE VARIATION OF DENSITIES AND SURFACE TENSIONS OF IRON-NICKEL MELTS*, 1969.

[49] WD Drotning, "Thermal Expansion of Nickel to 2300 K", *Thermal Expansion 7*, Springer, 1982, DOI: 10.1007/978-1-4684-8267-6_2.

[50] LD Lucas and Mem Sci Rev Met, "Density of Metals at High Temperatures in the Solid and Molten States, Part 2", *Mem. Sci. Rev. Met* (1972).

[51] VN Eremenko and VI Nizhenko, "Surface Tension of Nickel Based Liquid Alloys. 1. The Ni–Sn–Al2O3 System", *Ukrainskii Khimicheskii Zhurnal* (1964).

[52] S V Stankus and R A Khairulin, "Thermophysics of Metastable Liquids in Relation with the Phenomena of Boiling and Crystallization", Russian, *Book of Abstracts, All-Union Symposium*, Sverdlovsk, 1985.

[53] Sang K. Chung, David B. Thiessen, and Won-Kyu Rhim, "A noncontact measurement technique for the density and thermal expansion coefficient of solid and liquid materials", en, *Review of Scientific Instruments* (Sept. 1996), ISSN: 0034-6748, 1089-7623, DOI: 10.1063/1.1147584.

[54] Takehiko Ishikawa, Paul-Francois Paradis, and Yutaka Saita, "Thermophysical Property Measurements of Molten Nickel Using an Electrostatic Levitation Furnace", ja, *Journal of the Japan Institute of Metals* (2004), ISSN: 0021-4876, DOI: 10.2320/jinstmet.68.781.

[55] Hanbyeol Yoo, Cheolmin Park, Sangho Jeon, Sooheyong Lee, and Geun Woo Lee, "Uncertainty evaluation for density measurements of molten Ni, Zr, Nb and Hf by using a containerless method", *Metrologia* (Oct. 2015), ISSN: 0026-1394, 1681-7575, DOI: 10.1088/0026-1394/52/5/677.

[56] Hidekazu Kobatake and Jürgen Brillo, "Density and thermal expansion of Cr–Fe, Fe–Ni, and Cr–Ni binary liquid alloys", en, *Journal of Materials Science* (July 2013), ISSN: 0022-2461, 1573-4803, DOI: 10.1007/s10853-013-7274-0.

[57] J. Brillo, T. Schumacher, and K. Kajikawa, "Density of Liquid Ni-Ti and a New Optical Method for its Determination", en, *Metallurgical and Materials Transactions A* (Feb. 2019), ISSN: 1073-5623, 1543-1940, DOI: 10.1007/s11661-018-5047-8.

[58] Manabu Watanabe, Masayoshi Adachi, and Hiroyuki Fukuyama, "Densities of Fe–Ni melts and thermodynamic correlations", en, *Journal of Materials Science* (Apr. 2016), ISSN: 0022-2461, 1573-4803, DOI: 10.1007/s10853-015-9644-2.

[59] Shumpei Ozawa, Yu Kudo, Kazuhiko Kuribayashi, Yuki Watanabe, and Takehiko Ishikawa, "Precise density measurement of liquid titanium by electrostatic levitator", *Materials Transactions* (2017), DOI: 10.2320/matertrans.l-m2017835.

[60] Geun Woo Lee, Sangho Jeon, Cheolmin Park, and Dong-Hee Kang, "Crystal–liquid interfacial free energy and thermophysical properties of pure liquid Ti using electrostatic levitation: Hypercooling limit, specific heat, total hemispherical emissivity, density, and interfacial free energy", en, *The Journal of Chemical Thermodynamics* (Aug. 2013), ISSN: 00219614, DOI: 10.1016/j.jct.2013.03.012.

[61] Takehiko Ishikawa and Paul-François Paradis, "Thermophysical properties of molten refractory metals measured by an electrostatic levitator", *Journal of electronic materials* (2005), DOI: 10.1007/s11664-005-0160-z.

[62] Tunezo Saito, Yutaka Shiraishi, and Yutaka Sakuma, "Density measurement of molten metals by levitation technique at temperatures between 1800 and 2200 C", *Trans Iron Steel Inst Japan* (1969), DOI: 10.2355/isijinternational1966.9.118.

[63] Paul-François Paradis and Won-Kyu Rhim, "Non-contact measurements of thermophysical properties of titanium at high temperature", *The Journal of Chemical Thermodynamics* (2000), DOI: 10.1006/jcht.1999.0576.

[64] S. Jeon, D.-H. Kang, Y. H. Lee, S. Lee, and G. W. Lee, "Effect of atomic size on undercoolability of binary solid solution alloy liquids with Zr, Ti, and Hf using electrostatic levitation", en, *The Journal of Chemical Physics* (Nov. 2016), ISSN: 0021-9606, 1089-7690, DOI: 10.1063/1.4966649.

[65] S. Amore, S. Delsante, H. Kobatake, and J. Brillo, "Excess volume and heat of mixing in Cu-Ti liquid mixture", en, *The Journal of Chemical Physics* (Aug. 2013), ISSN: 0021-9606, 1089-7690, DOI: 10.1063/1.4817679.

[66] Manabu Watanabe, Masayoshi Adachi, and Hiroyuki Fukuyama, "Density measurement of Ti–X (X = Cu, Ni) melts and thermodynamic correlations", en, *Journal of Materials Science* (Mar. 2019), ISSN: 0022-2461, 1573-4803, DOI: 10.1007/s10853-018-3098-2.

[67] M Leitner and G Pottlacher, "Density of liquid niobium and tungsten and the estimation of critical point data", *Metallurgical and Materials Transactions A* (2019), DOI: 10.1007/s11661-019-05262-5.

[68] SV Koval', NI Kuskova, and SI Tkachenko, "Investigation of the mechanism of electric explosion of conductors and of the thermal characteristics of liquid metals", *Teplofizika vysokikh temperatur* (1997).

[69] H Hess, A Kloss, A Rakhel, and H Schneidenbach, "Determination of thermophysical properties of fluid metals by wire-explosion experiments", *International journal of thermophysics* (1999), DOI: 10.1023/a:1022635727340.

[70] T Hüpf, C Cagran, G Lohöfer, and G Pottlacher, "Electrical resistivity of high melting metals up into the liquid phase (V, Nb, Ta, Mo, W)", en, *Journal of Physics: Conference Series* (Feb. 2008), ISSN: 1742-6588, 1742-6596, DOI: 10.1088/1742-6596/98/6/062002.

[71] RS Hixson and MA Winkler, "Thermophysical properties of solid and liquid tungsten", *International Journal of Thermophysics* (1990), DOI: 10.1007/bf01184339.

[72] A Berthault, L Arles, and J Matricon, "High-pressure, high-temperature thermophysical measurements on tantalum and tungsten", *International journal of thermophysics* (1986), DOI: 10.1007/bf00503808.

[73] A Calverley, "A determination of the surface tension of liquid tungsten by the drop-weight method", *Proceedings of the Physical Society. Section B* (1957), DOI: 10.1088/0370-1301/70/11/303.

[74] Alexander Stukowski, "Visualization and analysis of atomistic simulation data with OVITO–the Open Visualization Tool", *Model. Simul. Mat. Sci. Eng.* (Jan. 2010), DOI: 10.1088/0965-0393/18/1/015012.

[75] Peter Mahler Larsen, Søren Schmidt, and Jakob Schiøtz, "Robust structural identification via polyhedral template matching", *Model. Simul. Mat. Sci. Eng.* (June 2016), DOI: 10.1088/0965-0393/24/5/055007.
